# Supplementary material for: On Prior Confidence and Belief Updating
Source: arXiv:2412.10662 source file (2025-05-14)
Supplement: Supplementary file 1 [file figure_supplement_interface.pdf]

**Comprehension Check**

Does the proportion of success and failure of projects vary across tasks?

- ○ Yes
- ○ No

Select all the statement(s) that is/are true about a test with 80% reliability?

- ☐ The test result will be Positive with 80% chance when the project is a success.
- ☐ The test result will be Positive with 80% chance when the project is a failure.
- ☐ The test result will be Negative with 80% chance when the project is a success.
- ☐ The test result will be Negative with 80% chance when the project is a failure.

Suppose a test has 80% reliability. After seeing a positive test result, the selected project is more likely to be a _____.

- ○ Success
- ○ Failure
- ○ Not possible to tell

The more confident I am of my guess being within 3 percentage points of the actual value, I should

- ○ Report a higher level of confidence
- ○ Report a lower level of confidence
- ○ What I report does not matter

------------------------------------------------------- Page Break -------------------------------------------------------

There are 100 projects arranged on a 10 by 10 grid.

- White Square = Success
- Black Square = Failure

Click the next button for the grid to appear on your screen.

---------------------------------------------------- Page Break ----------------------------------------------------

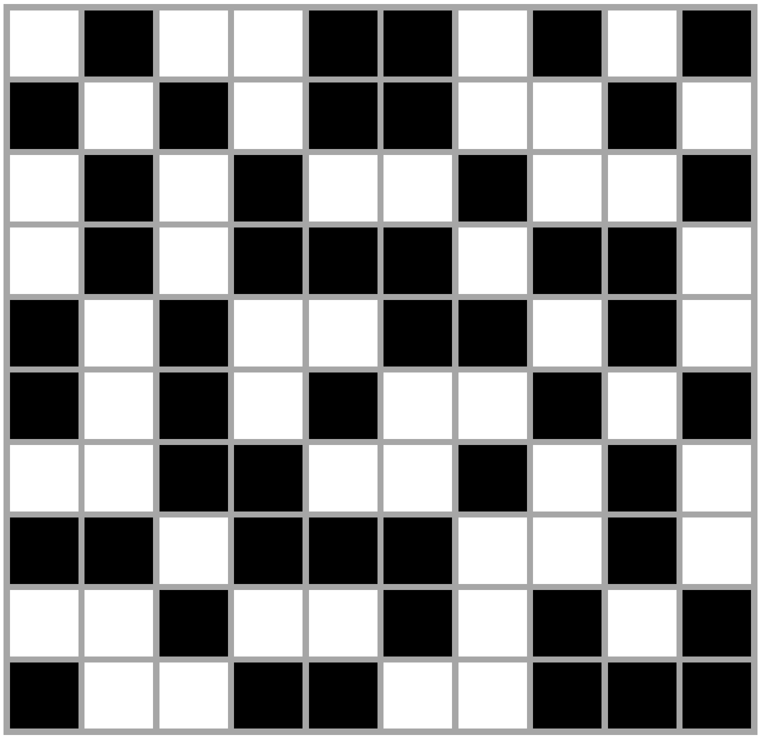

---------------------------------------------------- Page Break ----------------------------------------------------

One of the 100 projects is randomly selected for you to evaluate (with all projects having an equal chance of being selected). What is the chance that the selected project is a Success (white boxes)? Please input a number between 0-100 indicating the percentage of the project being a Success.

---------------------------------------------------- Page Break ----------------------------------------------------

You guessed that the chance of the randomly selected project is a success (white boxes) is _________%.

Please indicate the level of confidence, as a percentage between 0-100, you have that your guess is within 3 percentage points of the actual value.

[ ]

------------------------------------------------------- Page Break -------------------------------------------------------

Your guess that the randomly selected project is a success: _________%.

To further aid your assessment, the computer will run a test on the selected project. The test has a reliability of 80%, so it will be correct four times out of five.

- If the selected project is a Success, the test result will be Positive with 80% chance (four times out of five) and the test result will be Negative with 20% chance (one time out of five).
- If the selected project is a Failure, the test result will be Positive with 20% chance (one time out of five) and the test result will be Negative with 80% chance (four times out of five).

Test result: **Positive**

After seeing the test result, what is the chance that the selected project is a Success? Please input a number between **0-100** indicating the percentage of the project being a Success.

[ ]

------------------------------------------------------- Page Break -------------------------------------------------------

After seeing the test result, you guessed that the chance of the randomly selected project is a success (white boxes) is _________%.

Please indicate the level of confidence, as a percentage between 0-100, you have that your guess is within 3 percentage points of the statistical process.

[ ]
