# Supplementary material for: On Prior Confidence and Belief Updating
Source: arXiv:2412.10662 source file (2025-05-14)
Supplement: Supplementary file 2 [file figure_supplement_slides.pdf]

# WELCOME

- Welcome and thank you for participating in today's experiment.
- Please place all your personal belongings away so that we can have your complete attention.
- Please do not socialize or talk during the experiment.
- Please use the computers as instructed. Please do <u>not</u> attempt to browse the web or use programs unrelated to the experiment.
- You will be paid in private and with Venmo or Zelle at the end of the experiment.
- **The amount that you ultimately earn in the experiment depends on your decisions and chance.**

# TODAY'S EXPERIMENT IS ABOUT EVALUATING THE SUCCESS OF A PROJECT

- In this experiment, you are playing the role of a manager evaluating the chances of a selected project being a success.
- There are a total of 22 tasks with 4 different parts each, comprising of 2 guesses and 2 choices in the following order
  1. Guess
  2. Choice
  3. Guess
  4. Choice
- For every part, one of the tasks will be randomly selected for your payment. For example, you can be paid for your response in task 6 part 1, task 20 part 2 and so on.

# 1ST GUESS

- In every task, there are 100 projects, some of these projects are successes and others are failures.
  - The proportion of success and failures will vary across tasks.
  - The 100 projects are arranged on a 10 by 10 grid.
- Each project is represented by a square on the grid.
- The color of the square determines if the project is a success or a failure.
  - White Square = Success
  - Black Square = Failure
- For the first 11 tasks, the grid will be flashed on the screen for 0.25 seconds.

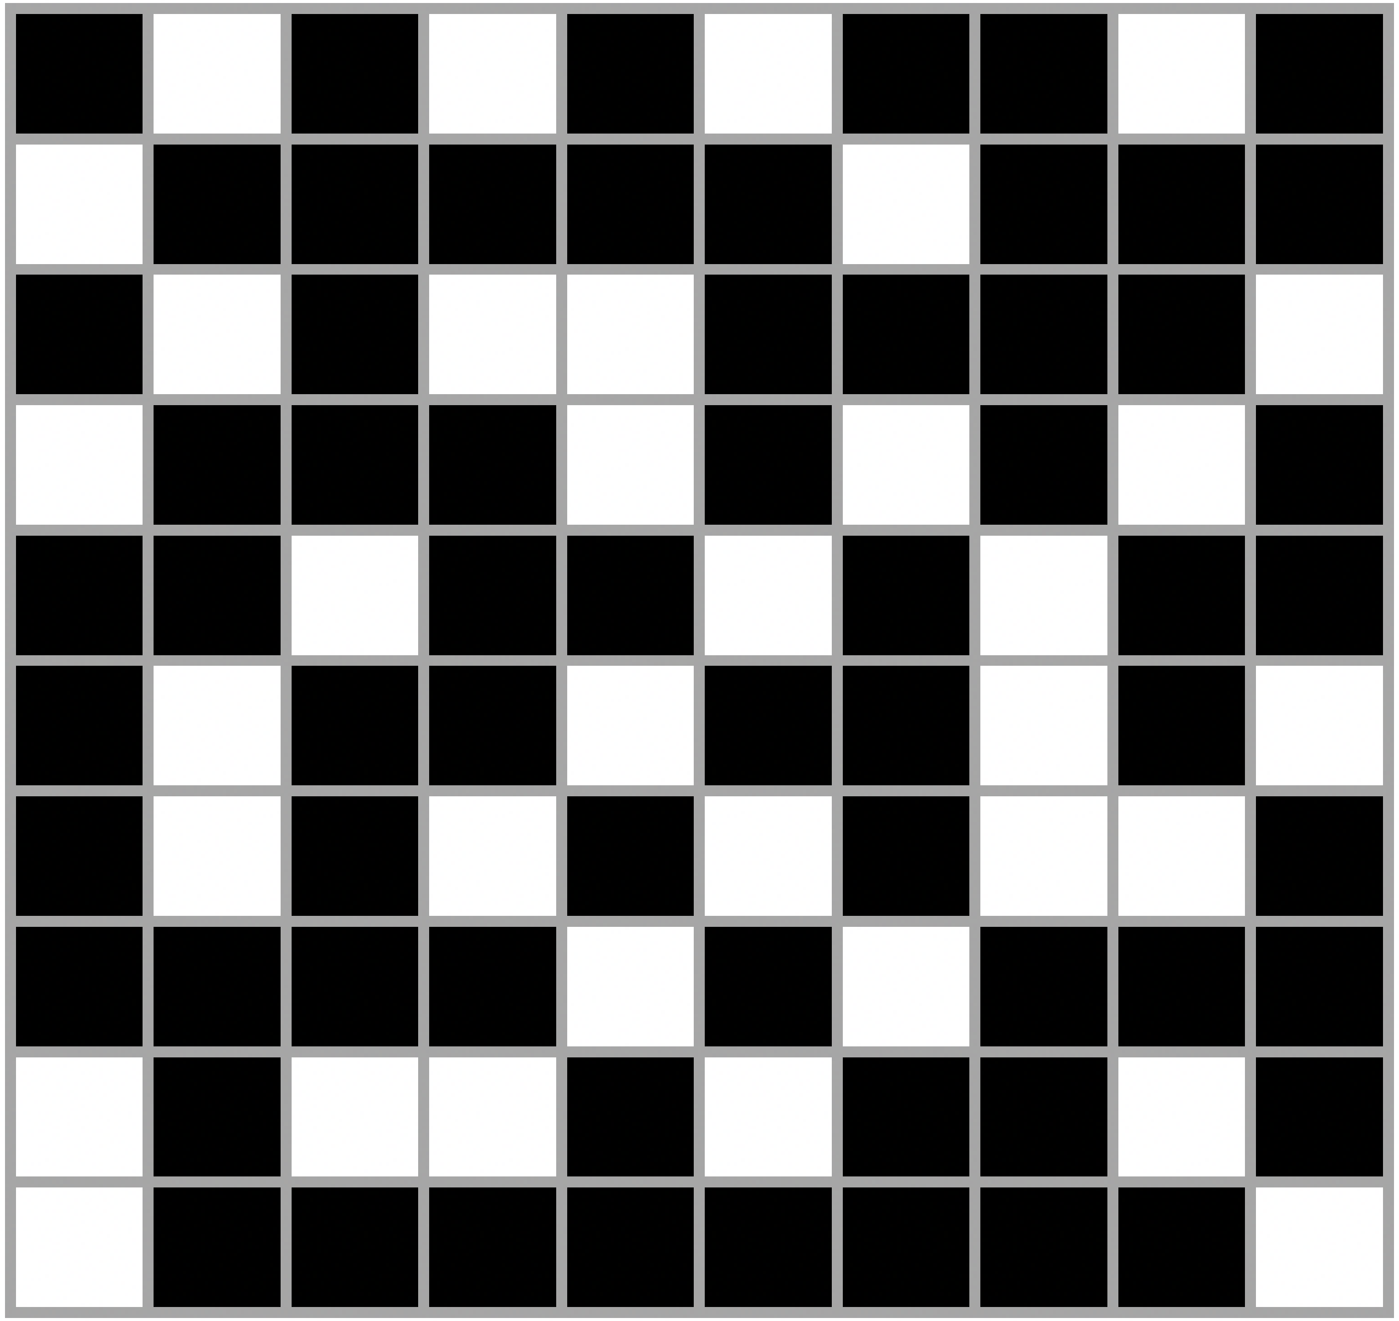

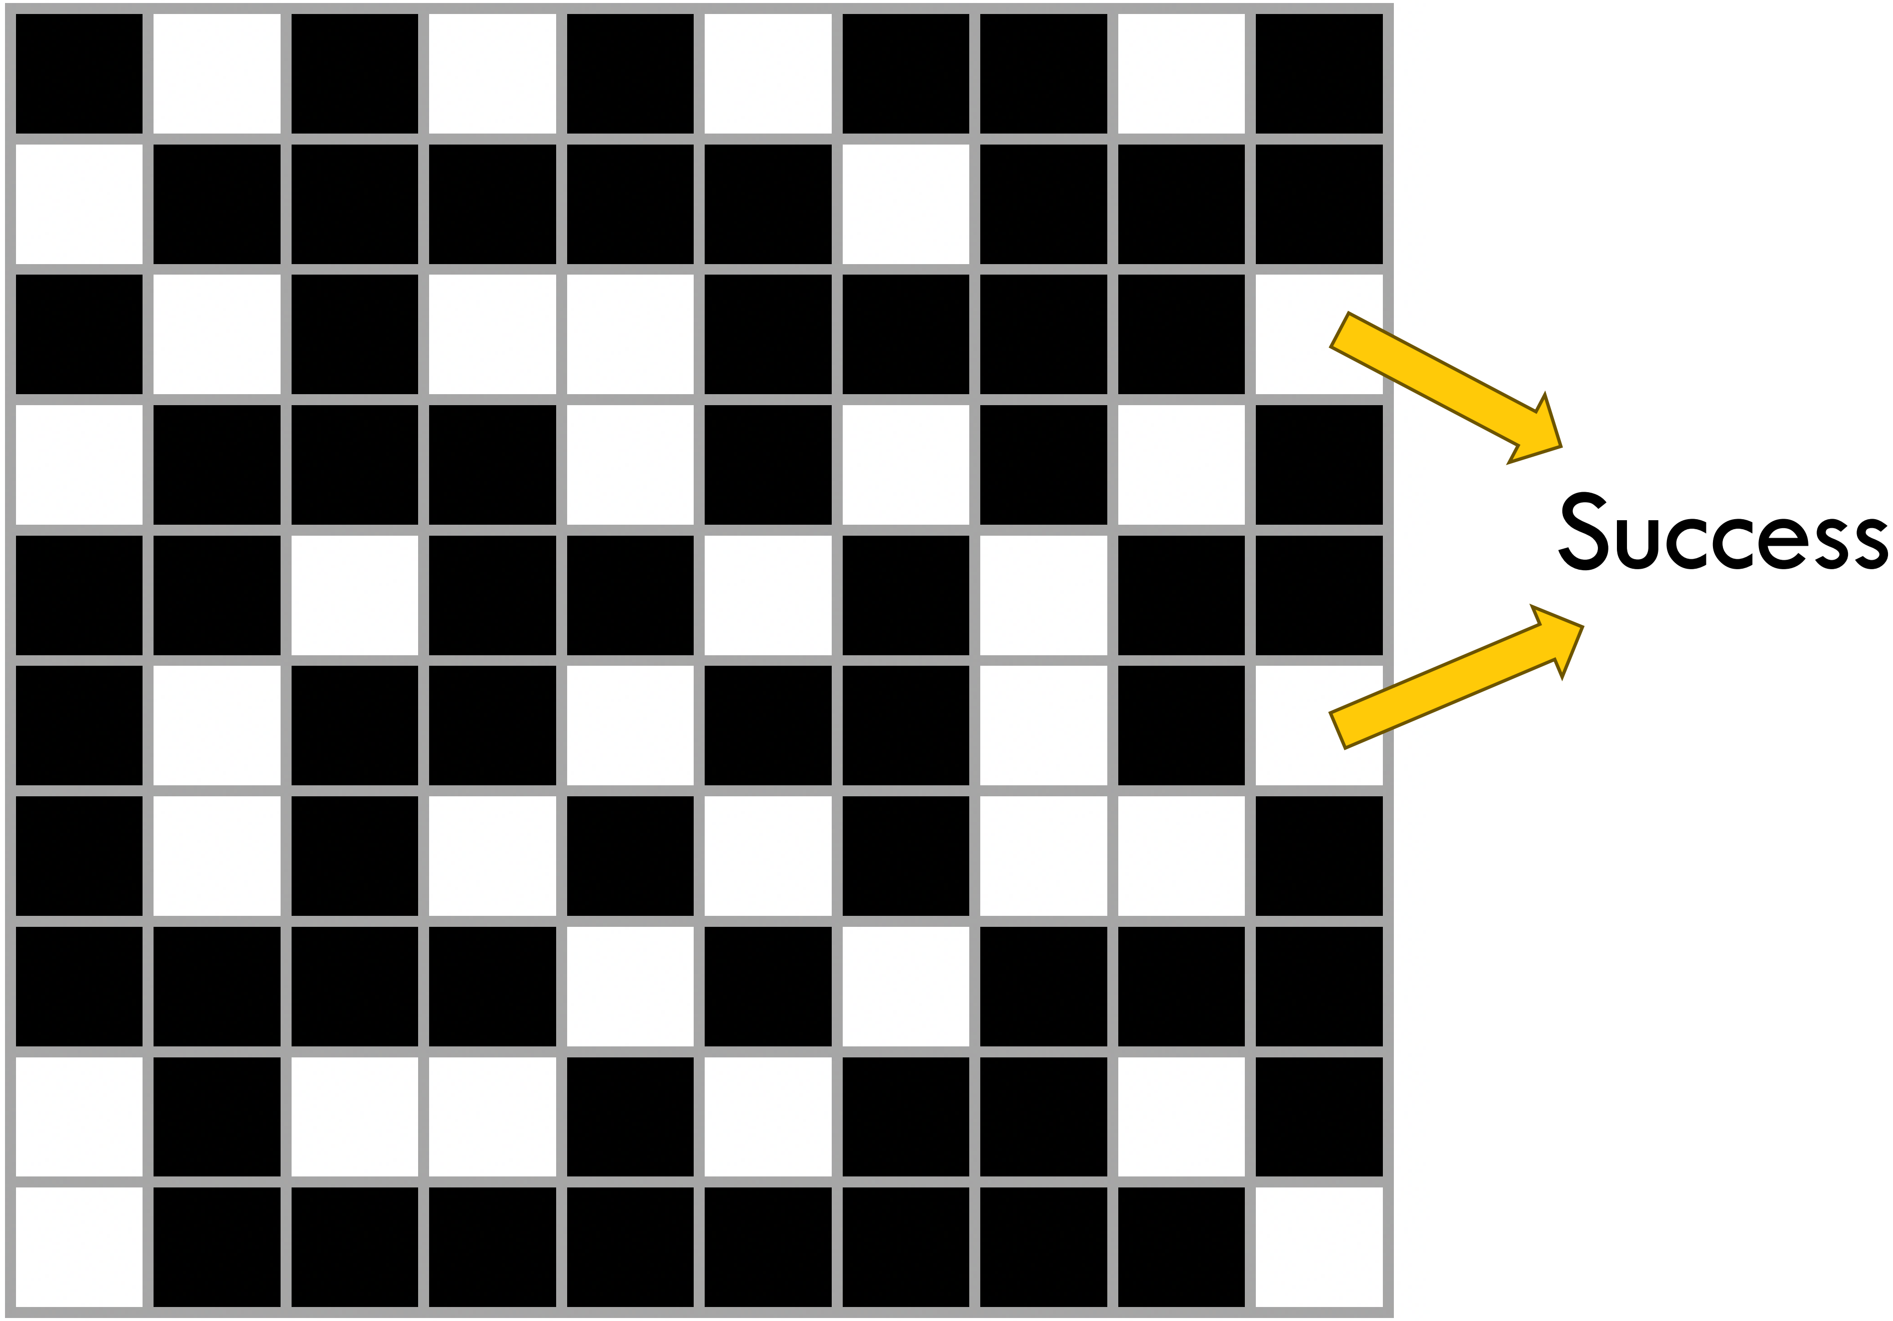
Success

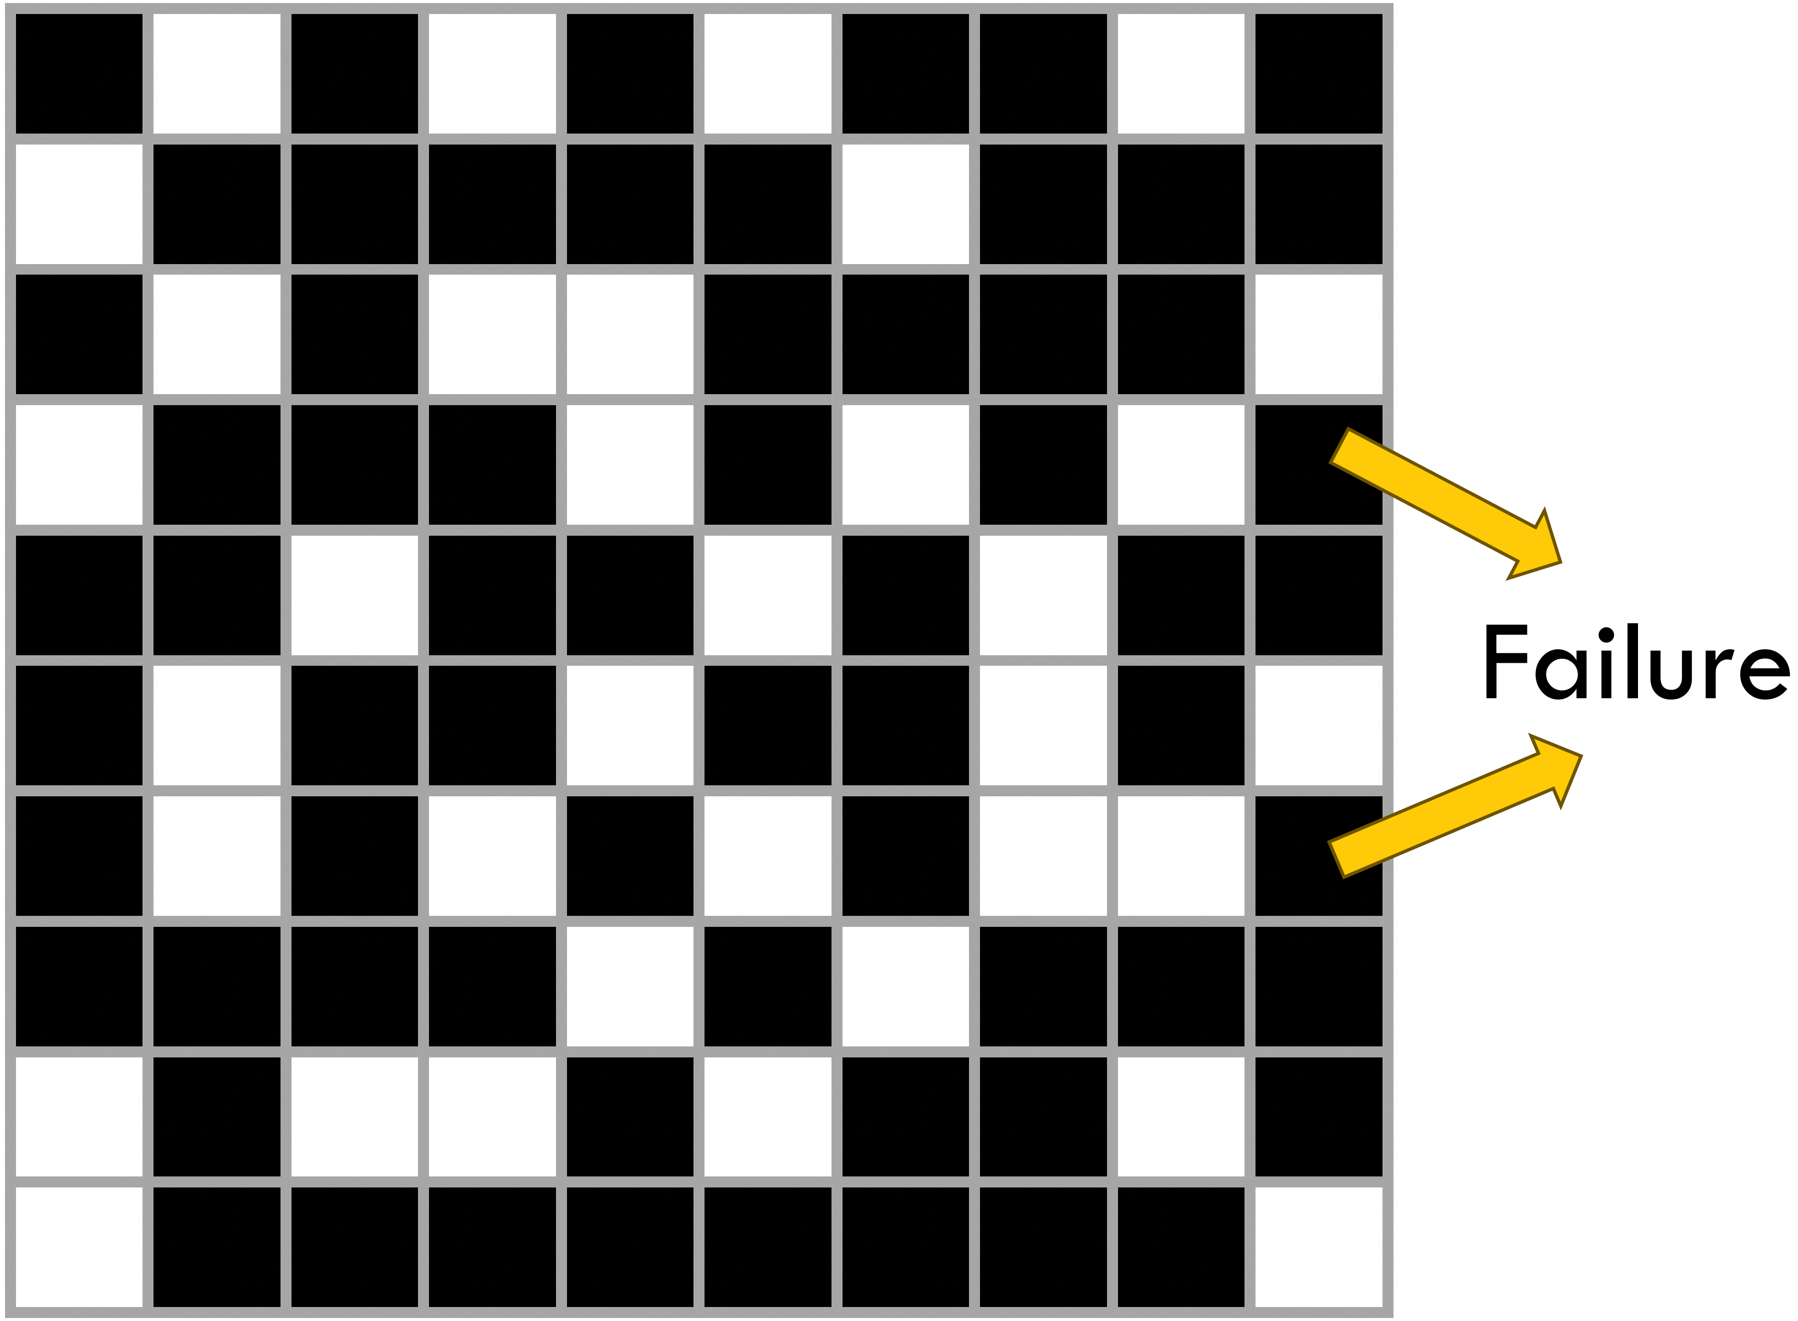
Failure

# 1ST GUESS

- One of the 100 projects from that grid is randomly selected for you to evaluate.
- With all projects having an **equal** chance of being selected.
- You will not know which specific project is selected.
- You will be asked to report the chance of the selected project being a success.

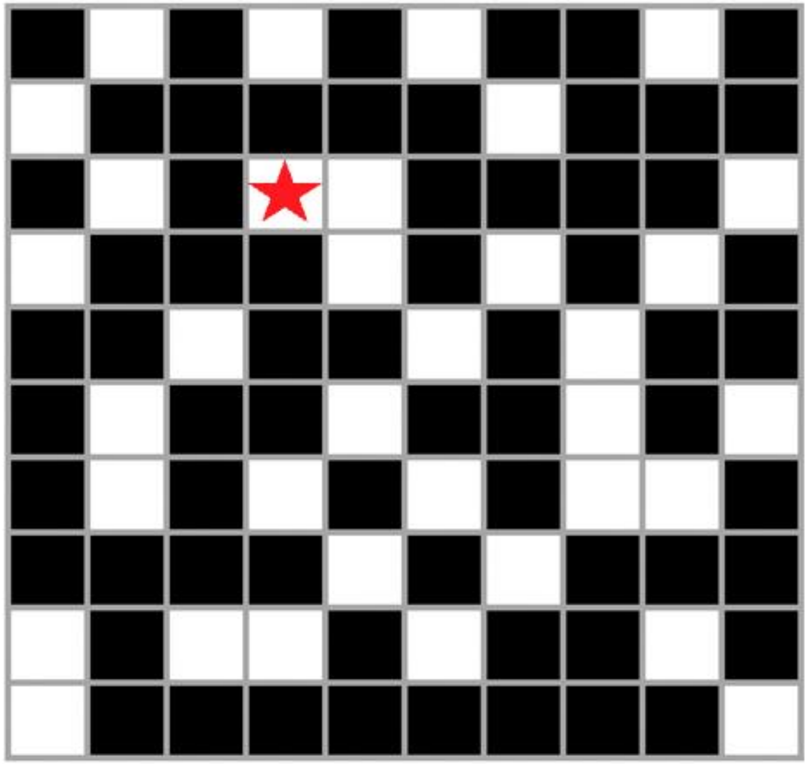

# 1$^{ST}$ GUESS

- For example, if you think there are 40 white squares
- This would mean 40% of the projects are successful (since there are 100 squares).
- There is a 40% chance that the randomly selected project is a success.
- You are not paid for whether the project is a success or a failure, but for how accurate you guess the chance of the selected project being a success.

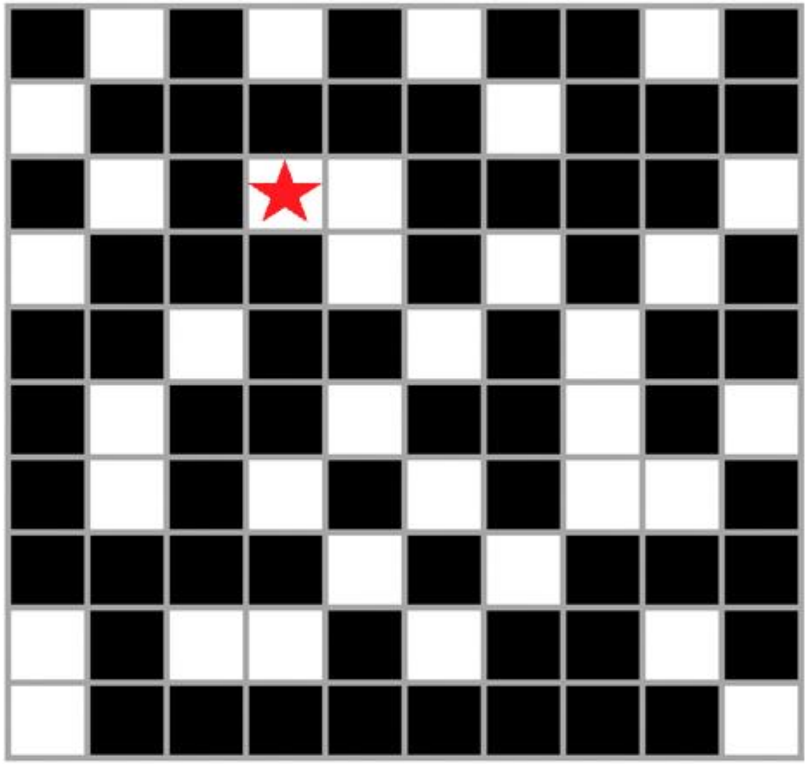

# 1$^{ST}$ GUESS

- For this part of each task, your earnings will be determined in the following manner:
- If your guess is **no more than 3 percentage points** from the actual value, you will **earn a bonus of $3** for this part.
- For example, if the actual value is 50%, you will earn a bonus of $3 if your response is between 47% and 53%, inclusive.

# 2ND GUESS

- To further aid your assessment on whether the selected project is a success or a failure:
- We will provide you with a computer test that has a reliability of 80% [60%].
- This test is not perfect. In 4 [3] out of 5 times, the computer will correctly predict whether the project is a success or a failure

# 2ND GUESS

- If the selected project is a Success, the test result will be Positive with 80% [60%] chance (four [three] times out of five) and the test result will be Negative with 20% [40%] chance (one [two] time out of five).
- If the selected project is a Failure, the test result will be Positive with 20% [40%] chance (one [two] time out of five) and the test result will be Negative with 80% [60%] chance (four [three] times out of five).
- You will be asked to report the chance of the selected project being a success after seeing the test result.

# 2ND GUESS

- For this part of each task, your earnings will be determined in the following manner:
- If your guess is **no more than 3 percentage points** from the value computed from a statistical process (we can show you this process after the experiment if you like), you will **earn a bonus of $3** for this part.
- For example, if the value computed from the statistical process is 50%, you will earn a bonus of $3 if your response is between 47% and 53%, inclusive.

# CHOICES

- We will now explain how the choices that follow each guess works.
- After you have submitted your guess, you will have the opportunity to win another $3 with the following choice you make:
- You will state your level of confidence (in percentage) that your guess is within 3 percentage points of the actual value or the statistical process.

# CHOICES

- We are going to ask you the following list of questions:

| Qn # | | Option A | | Option B |
|---|---|---|---|---|
| 1 | Would you rather have: | Stick to your guess | or | 0% chance of $3 |
| 2 | Would you rather have: | Stick to your guess | or | 1% chance of $3 |
| 3 | Would you rather have: | Stick to your guess | or | 2% chance of $3 |
| ⋮ | ⋮ | ⋮ | ⋮ | ⋮ |
| 100 | Would you rather have: | Stick to your guess | or | 99% chance of $3 |
| 101 | Would you rather have: | Stick to your guess | or | 100% chance of $3 |

# CHOICES

- If you choose Option A we will pay you **$3** for the choice if **your guess is within 3 percentage points** of the actual value/statistical process.
- If you choose Option B, you will be given a **lottery** that **pays $3** with the **stated chance** and nothing otherwise.

| Qn # | | Option A | | Option B |
|---|---|---|---|---|
| 1 | Would you rather have: | Stick to your guess | or | 0% chance of $3 |
| 2 | Would you rather have: | Stick to your guess | or | 1% chance of $3 |
| 3 | Would you rather have: | Stick to your guess | or | 2% chance of $3 |
| ⋮ | ⋮ | ⋮ | ⋮ | ⋮ |
| 100 | Would you rather have: | Stick to your guess | or | 99% chance of $3 |
| 101 | Would you rather have: | Stick to your guess | or | 100% chance of $3 |

# CHOICES

- After you answer all 101 questions, we will randomly pick one question and pay you the option you chose on that one question. Each question is equally likely to be chosen for payment.

| Qn # | | Option A | | Option B |
|---|---|---|---|---|
| 1 | Would you rather have: | Stick to your guess | or | 0% chance of $3 |
| 2 | Would you rather have: | Stick to your guess | or | 1% chance of $3 |
| 3 | Would you rather have: | Stick to your guess | or | 2% chance of $3 |
| ⋮ | ⋮ | ⋮ | ⋮ | ⋮ |
| 100 | Would you rather have: | Stick to your guess | or | 99% chance of $3 |
| 101 | Would you rather have: | Stick to your guess | or | 100% chance of $3 |

# CHOICES

- We suspect that you may choose Option A in at least the first few questions, but at some point will switch to choosing Option B.
- So, to save time, just tell us at which point you'd switch. We can then 'fill out' your answers to all 101 questions based on your switch point

| Qn # | | Option A | | Option B |
|---|---|---|---|---|
| 1 | Would you rather have: | Stick to your guess | or | 0% chance of $3 |
| 2 | Would you rather have: | Stick to your guess | or | 1% chance of $3 |
| 3 | Would you rather have: | Stick to your guess | or | 2% chance of $3 |
| ⋮ | ⋮ | ⋮ | ⋮ | ⋮ |
| 100 | Would you rather have: | Stick to your guess | or | 99% chance of $3 |
| 101 | Would you rather have: | Stick to your guess | or | 100% chance of $3 |

# CHOICES

- Suppose your switch point is 75
- We will choose option A for all the rows before 76
- We will choose option B for row 76 and any rows that come after

| Qn # | | Option A | | Option B |
|---|---|---|---|---|
| 1 | Would you rather have: | Stick to your guess | or | 0% chance of $3 |
| 2 | Would you rather have: | Stick to your guess | or | 1% chance of $3 |
| ⋮ | ⋮ | ⋮ | ⋮ | ⋮ |
| 76 | Would you rather have: | Stick to your guess | or | 75% chance of $3 |
| ⋮ | ⋮ | ⋮ | ⋮ | ⋮ |
| 101 | Would you rather have: | Stick to your guess | or | 100% chance of $3 |

# CHOICES

- This switch point is your level of confidence that your guess is within 3 percentage points of the actual value.

| Qn # | | Option A | | Option B |
|---|---|---|---|---|
| 1 | Would you rather have: | Stick to your guess | or | 0% chance of $3 |
| 2 | Would you rather have: | Stick to your guess | or | 1% chance of $3 |
| ⋮ | ⋮ | ⋮ | ⋮ | ⋮ |
| 76 | Would you rather have: | Stick to your guess | or | 75% chance of $3 |
| ⋮ | ⋮ | ⋮ | ⋮ | ⋮ |
| 101 | Would you rather have: | Stick to your guess | or | 100% chance of $3 |

# CHOICES

- If you are 75% confident that your guess is within 3 percentage points of the actual value, you should only be willing to accept lotteries that pay $3 at least 75% of the time.
- Reporting you are 75% confident will ensure you only get lotteries that pays $3 at least 75% of the time.

| Qn # | | Option A | | Option B |
|---|---|---|---|---|
| 1 | Would you rather have: | Stick to your guess | or | 0% chance of $3 |
| 2 | Would you rather have: | Stick to your guess | or | 1% chance of $3 |
| ⋮ | ⋮ | ⋮ | ⋮ | ⋮ |
| 76 | Would you rather have: | Stick to your guess | or | 75% chance of $3 |
| ⋮ | ⋮ | ⋮ | ⋮ | ⋮ |
| 101 | Would you rather have: | Stick to your guess | or | 100% chance of $3 |

# SUMMARY

- In summary, each task has 4 decisions that you will have to make in the following order:

1. Guess the chance that the selected project is a success after seeing the grid
2. State your confidence level for the earlier guess.
3. Guess the chance that the selected project is a success after seeing a test result
4. State your confidence level for the earlier guess.

- There are a total of 22 tasks in this experiment with 4 different parts each.
- For every part, one of the tasks will be randomly selected for your payment. For example, you can be paid for your response in task 6 part 1, task 20 part 2 and so on.

# SUMMARY

- For the first 11 tasks, the grid will be flashed on your screen for 0.25 seconds

- We will provide more information about the last 11 tasks later in the experiment

# EARNINGS FROM EXPERIMENT

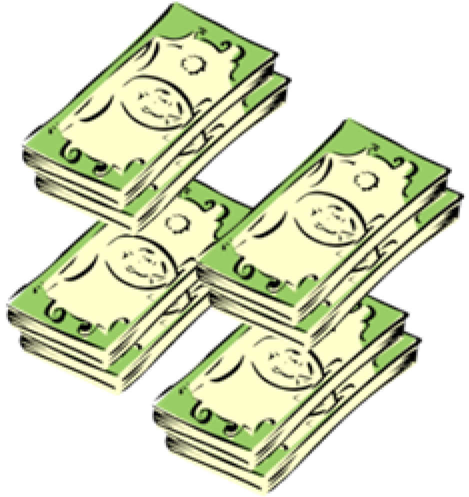

- You have already earned $7 for showing up on time.

- You will also receive earnings (in $) depending on the responses you have provided in this experiment.

**If there are no further questions, we will begin the experiment!**
